# Supplementary material for: Bridging the Gap: Categorizing Gravitational-Wave Events at the Transition Between Neutron Stars and Black Holes
Source: arXiv:2111.03498 source file (2022-07-13)
Supplement: Supplementary file 1 [file hyperparameters_appendix.tex]

\section{Hyperposteriors Inferred for \dipbreak}
\label{ap:hyperparams}

We list all hyperparameters and their priors for the \dipbreak{} model in Table~\ref{tab:hyperparams}. We additionally Supply 90\% CIs for their inferred posteriors.
\broken{} is parametrized similarly to  \dipbreak, but sets $A=0$, rendering $\glo$ and $\ghi$ meaningless. The prior on $\mbreak$ for \broken{} is U($1.4\,\Msun$, $3\,\Msun$).
\discontinuity{} also utilizes the same hyperparameters as \dipbreak, but sets $\eta_{\text{high}} = 0$, and the prior on $A$ becomes U($0,2$) because the allowed extent of a high-pass filter is 2, whereas the allowed extent of a notch filter (like that in \dipbreak) is 1. 

\begin{table}[t]
    \centering
    \begin{tabular}{ c  p{8cm} p{2mm} p{2.8cm} c }
        \hline\hline
        {\bf Parameter} & \textbf{Description} &  & \textbf{Prior} & \textbf{Posterior} \\\hline
        $\alpha_1$ & Spectral index for the power law of the mass distribution at low mass. &  & U($-4$, $12$) 
        & $\CIPlusMinus{\dipbreakMatterMattersBinnedPairing[param][alpha_1]}$ \\
        $\alpha_2$ & Spectral index for the power law of the mass distribution at high mass. &  & U($-4$, $12$) 
        & $\CIPlusMinus{\dipbreakMatterMattersBinnedPairing[param][alpha_2]}$ \\
        $\mathrm{A}$ & Lower mass gap depth. &  & U($0,1$)
        & $\CIPlusMinus{\dipbreakMatterMattersBinnedPairing[param][A]}$ \\
        $\gamma_{\rm low}$ & Location of lower end of the mass gap. &  & U($1.4\,\Msun$, $3\,\Msun$)
        & $\CIPlusMinus{\dipbreakMatterMattersBinnedPairing[param][NSmax]}$ \\
        $\gamma_{\rm high}$ & Location of upper end of the mass gap &  & U($3\,\Msun$, $9\,\Msun$) 
        & $\CIPlusMinus{\dipbreakMatterMattersBinnedPairing[param][BHmin]}$ \\
        $\eta_{\text{low}}$ & Steepness of the lower end of the mass gap. &  & 50 
        & \mdash{} \\
        $\eta_{\text{high}}$ & Steepness of the upper end of the mass gap. &  & 50 
        & \mdash{} \\
        $\eta$ & Parameter controlling tapering of the power law at high mass &  & U($-4$, $12$) 
        &$\CIPlusMinus{\dipbreakMatterMattersBinnedPairing[param][n3]}$ \\
        $m_{\rm break}$ & Break in the power law between $\alpha_1$ and $\alpha_2$ &  & Fixed at $\gamma_{\rm low}$
        & \mdash{} \\
        $\beta_1$ & Spectral index for the power-law-in-mass-ratio pairing function for secondary masses below $5 \Msun$. &  & U($-4$, $12$)  
        &$\CIPlusMinus{\dipbreakMatterMattersBinnedPairing[param][beta_q_1]}$ \\
        $\beta_2$ & Spectral index for the power-law-in-mass-ratio pairing function for secondary masses above $5 \Msun$. &  & U($-4$, $12$)  
        &$\CIPlusMinus{\dipbreakMatterMattersBinnedPairing[param][beta_q_2]}$ \\
        $m_{\text{min}}$ & Minimum mass of the power-law component of the mass distribution. &  & U($1\, \Msun$, $1.4\, \Msun$)
        &$\CIPlusMinus{\dipbreakMatterMattersBinnedPairing[param][NSmin]}$ \\
        $\mmax$ &  Maximum mass of the power-law component of the mass distribution. &  & U($30\, \Msun$, $100\, \Msun$)
        &$\CIPlusMinus{\dipbreakMatterMattersBinnedPairing[param][BHmax]}$ \\
        \hline\hline
    \end{tabular}
    \caption{\label{tab:hyperparams} Table of all hyperparameters, their priors, and their inferred posteriors under the \dipbreak{} model. Errors are quoted as 90\% credible intervals.}
\end{table}
