# Supplementary material for: Bridging the Gap: Categorizing Gravitational-Wave Events at the Transition Between Neutron Stars and Black Holes
Source: arXiv:2111.03498 source file (2022-07-13)
Supplement: Supplementary file 2 [file rates_from_injections_appendix.tex]

\section{Estimating Rates from Monte-Carlo Integrals over Injected GW Signals}
\label{sec:rates_from_injs}
We start off with a decomposition of the intrinsic merger rate distribution such that
\begin{equation}
    \frac{dN}{dm_1 dm_2 d\vec{s}_1 d\vec{s}_2 d\vec{\Omega} dz dt_\mathrm{det}} = \mathcal{N} p(m_1, m_2, \vec{s}_1, \vec{s}_2, \vec{\Omega}|z) f(z) \frac{dV_c}{dz}\frac{1}{1+z} \left( \int dz\, f(z) \frac{dV_c}{dz}\frac{1}{1+z} \right)^{-1} %\nonumber
\end{equation}
where we have assumed $\int dm_1 dm_2 d\vec{s}_1 d\vec{s}_2 d\vec{\Omega} \, p(m_1, m_2, \vec{s}_1, \vec{s}_2, \vec{\Omega}|z) = 1\ \forall\ z$.
Here, $m_{1,2}$ denote the source-frame component masses, $\vec{s}_{1,2}$ denote the component spins, $\vec{\Omega}$ denotes the entire set of angles determining the source position (RA, Dec, inclination, and polarization angle) and $z$ the redshift at which the merger occurs.
These single-event parameters completely describe quasi-circular binary black hole mergers; although additional parameters may be needed to describe eccentricity, matter effects, and/or alternate theories of gravity.

With this decomposition, we denote the distribution of events at a particular redshift (but not the total rate) by $p(m_1, m_2, \vec{s}_1, \vec{s}_2, \vec{\Omega}|z)$ while the total rate (per unit comoving volume per unit source-frame time) at a particular redshift is set by $\mathcal{N} f(z)$.
We also note that the expected number of detections is given by
\begin{equation}
    \mathcal{E} = \int dm_1 dm_2 d\vec{s}_1 d\vec{s}_2 d\vec{\Omega} dz dt_\mathrm{det}\, \left(\frac{dN}{dm_1 dm_2 d\vec{s}_1 d\vec{s}_2 d\vec{\Omega} dz dt_\mathrm{det}}\right) P(\mathrm{det}|t_\mathrm{det}, m_1, m_2, \vec{s}_1, \vec{s}_2, \vec{\Omega}, z) %\nonumber
\end{equation}
and is related to the observed number of events ($N_\mathrm{obs}$) via $\mathcal{E} \sim p(N_\mathrm{obs}|\mathcal{E})p(\mathcal{E}) = \mathcal{E}^{N_\mathrm{obs}} e^{-\mathcal{E}} / \mathcal{E}$.
In this expression, $P(\mathrm{det}|t_\mathrm{det}, m_1, m_2, \vec{s}_1, \vec{s}_2, \vec{\Omega}, z)$ is the probability of detecting a signal at time $t_\mathrm{det}$ with the specified parameters obtained by marginalizing over possible noise realizations for which the source is detectable.
The likelihood for observing $N_\mathrm{obs}$ events with an expected number of $\mathcal{E}$ is Poisson and, although not strictly necessary, a prior for the overall normalization that is flat in $\log \mathcal{E}$ is often assumed when sampling from the posterior for the population distribution after marginalizing over the rate.
The choice of prior needs to be enforced consistently.

Now, we can approximate the integrals with estimators for $\mathcal{E}$ from Monte-Carlo sample sets drawn from
\begin{gather}
    m_1,\ m_2, \vec{s}_1, \vec{s}_2, \vec{\Omega} \sim p_\mathrm{draw}(m_1, m_2, \vec{s}_1, \vec{s}_2, \vec{\Omega}|z) \nonumber \\
    z \sim \left(\frac{dV_c}{dz} \frac{1}{1+z}\right) f_\mathrm{draw}(z) %\nonumber
\end{gather}
(which implicitly assumes that events are distributed uniformly in detector-frame time) with the following
\begin{align}
    \mathcal{E} & = \int dt_\mathrm{det} dz dm_1 dm_2 d\vec{s}_1 d\vec{s}_2 d\vec{\Omega}\, \left[ \mathcal{N} p(m_1, m_2, \vec{s}_1, \vec{s}_2, \vec{\Omega}|z) f(z) \frac{dV_c}{dz}\frac{1}{1+z} \left( \int dz\, f(z) \frac{dV_c}{dz}\frac{1}{1+z} \right)^{-1} \right. \nonumber \\
                & \quad\quad\quad\quad\quad\quad\quad\quad\quad\quad\quad\quad\quad\quad\quad\quad\quad\quad\quad\quad\quad\quad\quad\quad\quad\quad\quad\quad \left. \times P(\mathrm{det}|t_\mathrm{det}, m_1, m_2, \vec{s}_1, \vec{s}_2, \vec{\Omega}, z) \right] \nonumber \\
                & = \int dz dm_1 dm_2 d\vec{s}_1 d\vec{s}_2 d\vec{\Omega}\, \left[ \mathcal{N} p(m_1, m_2, \vec{s}_1, \vec{s}_2, \vec{\Omega}|z) f(z) \frac{dV_c}{dz}\frac{1}{1+z} \left( \int dz\, f(z) \frac{dV_c}{dz}\frac{1}{1+z} \right)^{-1} \right. \nonumber \\
                &  \quad\quad\quad\quad\quad\quad\quad\quad\quad\quad\quad\quad\quad\quad\quad\quad\quad\quad\quad\quad\quad\quad\quad\quad\quad \times \left. \int dt_\mathrm{det}\, P(\mathrm{det}|t_\mathrm{det}, m_1, m_2, \vec{s}_1, \vec{s}_2, \vec{\Omega}, z) \right] % \nonumber
\end{align}
\begin{align}
    \mathcal{E} & = \int dz dm_1 dm_2 d\vec{s}_1 d\vec{s}_2 d\vec{\Omega}\, \left[ \mathcal{N} p(m_1, m_2, \vec{s}_1, \vec{s}_2, \vec{\Omega}|z) f(z) \frac{dV_c}{dz}\frac{1}{1+z} \left( \int dz\, f(z) \frac{dV_c}{dz}\frac{1}{1+z} \right)^{-1} \right. \nonumber \\
                &  \quad\quad\quad\quad\quad\quad\quad\quad\quad\quad\quad\quad\quad\quad\quad\quad\quad\quad\quad\quad\quad\quad\quad\quad \left. \times T_\mathrm{det} \left<P(\mathrm{det}|t_\mathrm{det}, m_1, m_2, \vec{s}_1, \vec{s}_2, \vec{\Omega}, z)\right>_{T_\mathrm{det}} \right] \nonumber \\
                & \approx T_\mathrm{det} \left(N_\mathrm{inj}^{-1} \sum\limits_\mathrm{found}^{N_\mathrm{fnd}} \frac{ \mathcal{N} p(m_1, m_2, \vec{s}_1, \vec{s}_2, \vec{\Omega}|z) f(z) (dV_c/dz)(1+z)^{-1} \left( \int dz\, f(z) (dV_c/dz) (1+z)^{-1} \right)^{-1} }{p_\mathrm{draw}(m_1, m_2, \vec{s}_1, \vec{s}_2, \vec{\Omega}|z) f_\mathrm{draw}(z) (dV_c/dz) (1+z)^{-1} \left( \int dz\, f_\mathrm{draw}(z)(dV_c/dz)(1+z)^{-1}\right)^{-1}}\right) \nonumber \\
                & = \left(T_\mathrm{det} \int dz\, f_\mathrm{draw}(z) \frac{dV_c}{dz} (1+z)^{-1}\right) \left(\frac{\mathcal{N}}{\int dz\, f(z) (dV_c/dz) (1+z)^{-1}} \right) \left( N_\mathrm{inj}^{-1} \sum\limits_\mathrm{found}^{N_\mathrm{fnd}} \frac{p(m_1, m_2, \vec{s}_1, \vec{s}_2, \vec{\Omega}|z) f(z)}{p_\mathrm{draw}(m_1, m_2, \vec{s}_1, \vec{s}_2, \vec{\Omega}|z)f_\mathrm{draw}(z)} \right) %\nonumber
\end{align}
where we approximate $\left<P(\mathrm{det}|m_1, m_2, \vec{s}_1, \vec{s}_2, \vec{\Omega})\right>_{T_\mathrm{det}}$ with a sum over the $N_\mathrm{fnd}$ detected injections out of $N_\mathrm{inj}$ total injections that were uniformly distributed in detector-frame time.
This implies
\begin{multline}
    \frac{\mathcal{N}}{\int dz\, f(z) (dV_c/dz) (1+z)^{-1}} = \left( \frac{\mathcal{E}}{T_\mathrm{det} \int dz\, f_\mathrm{draw}(z) (dV_c/dz) (1+z)^{-1}}\right) \\ \times \left( N_\mathrm{inj}^{-1} \sum\limits_\mathrm{found}^{N_\mathrm{fnd}} \frac{p(m_1, m_2, \vec{s}_1, \vec{s}_2, \vec{\Omega}|z) f(z)}{p_\mathrm{draw}(m_1, m_2, \vec{s}_1, \vec{s}_2, \vec{\Omega}|z) f_\mathrm{draw}(z)} \right)^{-1} %\nonumber
\end{multline}
Furthermore, the quantity of immediate interest is the rate density at a particular redshift (e.g., $z=0$) per unit source-frame time, which is
\begin{align}
    \frac{dN}{dV_c dt_\mathrm{src}}(z) & = \left(\frac{dV_c}{dz}\right)^{-1} \frac{dt_\mathrm{det}}{dt_\mathrm{src}} \int dm_1 dm_2 d\vec{s}_1 d\vec{s}_2 d\vec{\Omega}\, \left( \frac{dN}{dm_1 dm_2 d\vec{s}_1 d\vec{s}_2 d\vec{\Omega} dz dt_\mathrm{det}} \right) \nonumber \\
                                    & = f(z) \left(\frac{\mathcal{N}}{\int dz\, f(z) (dV_c/dz)(1+z)^{-1}}\right) \int dm_1 dm_2 d\vec{s}_1 d\vec{s}_2 d\vec{\Omega}\, p(m_1, m_2, \vec{s}_1, \vec{s}_2, \vec{\Omega}|z) \nonumber \\
                                    & \approx f(z) \left(\frac{\mathcal{E}}{T_\mathrm{det} \int dz\, f_\mathrm{draw}(z) (dV_c/dz) (1+z)^{-1}}\right) \left( N_\mathrm{inj}^{-1} \sum\limits_\mathrm{found}^{N_\mathrm{fnd}} \frac{p(m_1, m_2, \vec{s}_1, \vec{s}_2, \vec{\Omega}|z) f(z)}{p_\mathrm{draw}(m_1, m_2, \vec{s}_1, \vec{s}_2, \vec{\Omega}|z) f_\mathrm{draw}(z)} \right)^{-1} %\nonumber
\end{align}
Summing the distribution of $dN/dV_c dt_\mathrm{src}$ for each set of population paramters in our posterior distributions will yield our over-all estimate for the rate density distribution.

We note that $f(z)$ can be scaled by an arbitray multiplicative constant without changing the result, which is to be expected as we enforce proper normalization of the intrinsic rate density explicitly.
Without loss of generality, then, we often take $f(z=0)=1$ for convenience.
%We also note that the normalization term required for this calculation, then, only depends on the injected distribution; it can be computed once and stored alongside the list of detected injections.
%Although not required, one can scale $f_\mathrm{draw}$ to make
%\begin{equation}
%    T_\mathrm{det} \int dz\, f_\mathrm{draw}(z) \frac{dV_c}{dz}\left(\frac{1}{1+z}\right) = 1 %\nonumber
%\end{equation}
%and record the value of
%\begin{equation}
%    w_\mathrm{draw}(m_1, m_2, \vec{s}_1, \vec{s}_2, \vec{\Omega}, z) = p_\mathrm{draw}(m_1, m_2, \vec{s}_1, \vec{s}_2, \vec{\Omega}|z) f_\mathrm{draw}(z) %\nonumber
%\end{equation}
%for each injection, which simplifies the expression to
%\begin{equation}
%    \frac{dN}{dV_c dt_\mathrm{src}}(z) \approx f(z) \left( N_\mathrm{inj}^{-1} \sum\limits_\mathrm{found}^{N_\mathrm{fnd}} \frac{p(m_1, m_2, \vec{s}_1, \vec{s}_2, \vec{\Omega}|z)f(z)}{w_\mathrm{draw}(m_1, m_2, \vec{s}_1, \vec{s}_2, \vec{\Omega}, z)}\right)^{-1} %\nonumber
%\end{equation}
%This is distills the required information about each injection (beyond the values of the single-event parameters) to a single number: $w_\mathrm{draw}$.
%Additionally, if a fixed population that exactly matches the injected distribution is assumed, then this expression simplifies to
%\begin{equation}
%    \frac{dN}{dV_c dt_\mathrm{src}}(z) = \left(\frac{N_\mathrm{inj}}{N_\mathrm{found}}\right) f(z) \mathcal{E} %\nonumber
%\end{equation}
%where $\mathcal{E} \sim \mathcal{E}^{N_\mathrm{obs}-1} e^{-\mathcal{E}}$
%In what follows, we retain the normalization term as this choice for $f_\mathrm{draw}$ is not required.

The procedure to draw samples for $\mathcal{R}(z) = dN/dV_c dt_\mathrm{src}$ is therefore as follows.
For each hyper-parameter set drawn from the population distribution posterior
\begin{enumerate}
    \item compute $\mu  = N_\mathrm{inj}^{-1} \sum\limits_\mathrm{found}^{N_\mathrm{fnd}} \frac{p(m_1, m_2, \vec{s}_1, \vec{s}_2, \vec{\Omega}|z) f(z)}{p_\mathrm{draw}(m_1, m_2, \vec{s}_1, \vec{s}_2, \vec{\Omega}|z) f_\mathrm{draw}(z)} $
        \begin{itemize}
            \item if the population is assumed to be fixed to the same distribution used to generate the injections, this simplifies to $\mu = N_\mathrm{fnd}/ N_\mathrm{inj}$
        \end{itemize}
    \item draw enough samples for $\mathcal{E} \sim p(N_\mathrm{obs}|\mathcal{E}) p(\mathcal{E}) \sim \mathcal{E}^{N_\mathrm{obs}}e^{-\mathcal{E}} / \mathcal{E}$
        \begin{itemize}
            \item we assume a flat in $\log \mathcal{E}$ prior which is the assumption that was enforced when separating the population likelihood into the rate and shape parameters.
        \end{itemize}
    \item divide each $\mathcal{E}$ sample by a $\mu$ sample
    \item divide by the surveyed spacetime volume $T_\mathrm{det} \int dz\, f_\mathrm{draw}(z) (dV_c/dz) (1+z)^{-1}$
    \item multiply by $f(z)$
\end{enumerate}
Concatenting the result from all population hyper-parameter samples yields a set of samples for the rate.
